# Supplementary material for: Learning Audio-guided Video Representation with Gated Attention for Video-Text Retrieval
Source: arXiv:2504.02397 source file (2025-04-03)
Supplement: Supplementary file 3 [file supp_table_ablation.tex]

\begin{table}[!t]
% \vspace{-5mm}
\setlength{\tabcolsep}{2pt}
\fontsize{8.2}{9}\selectfont
\centering
\scalebox{0.95}{
\begin{tabularx}{0.499\textwidth}
    {
      >{\centering\arraybackslash}p{0.13\textwidth}
      >{\centering\arraybackslash}X
      >{\centering\arraybackslash}X
      >{\centering\arraybackslash}X
      }
     \toprule
    \multirow{1}{*}[-4.5mm]{\textbf{Ablated Setting}} & \multicolumn{3}{c}{\textbf{Text-to-Video Retrieval}} \\ [-0.3ex] \cmidrule(lr){2-4}  
    &  R@1 & R@5 & R@10   \\  [-0.4ex] \midrule
    \multicolumn{4}{l}{\textit{\textbf{(a) Layer depth of Gated Fusion Transformer: $L$}}} \\ [-0.3ex]\midrule
    $L$=1 & 49.0 & 74.0 & 82.6 \\
    $L$=2  & 49.8 & 74.0 & 83.0 \\
    \ccol$L$=4  &\ccol 50.2 &\ccol  74.3 & \ccol 83.2 \\
    $L$=6  & 49.5 & 74.2 & 82.6 \\    [-0.3ex]\midrule
    \multicolumn{4}{l}{\textit{\textbf{(b) Scaling factor in Eq.(5): $\lambda$}}} \\ [-0.3ex]\midrule
    $\lambda$=0.0 & 48.0 & 75.1 & 83.4 \\
    $\lambda$=0.1 & 49.4 & 74.8 & 83.8 \\
    \ccol$\lambda$=0.2  &\ccol 50.2 &\ccol  74.3 & \ccol 83.2 \\
    $\lambda$=0.3  & 50.0 & 74.4 & 83.2 \\    [-0.3ex]\midrule
    \multicolumn{4}{l}{\textit{\textbf{(c) Maximum margin in Eq.(5): $\delta$}}} \\ [-0.3ex]\midrule
    $\delta$=0.00 & 48.0 & 75.1 & 83.4 \\
    $\delta$=0.05 & 49.4 & 75.1 & 83.6 \\
    \ccol$\delta$=0.10  &\ccol 50.2 &\ccol  74.3 & \ccol 83.2 \\
    $\delta$=0.15 & 49.3 & 74.8 & 83.8 \\
    $\delta$=0.20  & 48.3 & 74.4 & 83.9 \\  [-0.3ex]\midrule
    \multicolumn{4}{l}{\textit{\textbf{(d) Gate mechanism type}}} \\ [-0.3ex]\midrule
    Hard Gate & 49.3 & 75.0 & 82.5 \\
    \ccol Soft Gate  &\ccol 50.2 &\ccol  74.3 & \ccol 83.2 \\
[-0.3ex]\bottomrule 
\end{tabularx}
}
\vspace{-1.5mm}
\caption{Ablation studies on hyperparameters. 
\colorbox{grey}{{gray}} corresponds to our default setting.
}
\label{tab:supp_ablation_hyp}
\vspace{-4mm}
\end{table}
